# Supplementary material for: Computing Euclidean k-Center over Sliding Windows
Source: arXiv:2001.01035 source file (2020-01-04)
Supplement: Supplementary file 1 [file appendix.tex]

%\newpage
\appendix
